# Supplementary material for: The FIDS Theorems: Tensions between Multinode and Multicore Performance in Transactional Systems
Source: arXiv:2308.03919 source file (2023-08-07)
Supplement: Supplementary file 1 [file formal_model.tex]

\section{Formal model}
\label{appendix:formal_model}

We consider an asynchronous \emph{message-passing} model among $n$ \emph{nodes} and any number of \emph{clients}. Each node has $k$ \emph{processes}.
%\Naama{Switched between k and n here, since we later use $n-f$ which is the standard notation for fault tolerance; for that, we need $n$ to be the number of nodes.}
Messages are sent either between two processes on different nodes or between a client and a process, and can be arbitrarily delayed or dropped. Processes handle messages one at a time. Furthermore, processes within one node communicate with each other via \emph{shared memory}. Each process also has access to it own \emph{private memory}, which is not accessible to any other process. We consider the problem of implementing a \emph{parallel distributed transactional system} (PDTS), which provides transactions operating on data that can reside at multiple nodes.

\smallskip\noindent
\textbf{Transactions.}
Transactions are executed on a database composed of a set of \emph{data items}, $\Sigma$, which can be accessed by \emph{read} and \emph{write} operations. Each node $i$ holds some subset $\Sigma_i \subseteq \Sigma$, which may overlap with the set held on other nodes. A \emph{transaction}, $T$, is a sequence of read and write operations on a subset of the data items called its \emph{data set}, $D_T \in \Sigma$. A transaction $T$'s \emph{write set}, $W_T \subseteq D_T$, is the set of data items that it writes, and analogously, $T$'s \emph{read set}, $R_T \subseteq D_T$, is the set of data items it reads. Two transactions are said to \emph{conflict} if their data sets intersect at an item that is in the write set of at least one of them.

\smallskip\noindent
\textbf{Implementations.} An \emph{implementation} of a PDTS provides data representation for transactions and data items, and algorithms specifying the behaviour of all processes and clients processing transactions. Clients implement the common transactional interface -- the begin(t), read(t, key), write(t, key), commit(t), abort(t) operations. We assume that each client executes one transaction at a time and can choose which process to communicate with on each node. Clients and processes communicate through the send(m)/receive(m) interface. We assume that each process solely executes one \emph{message handler} at a time, triggered by receive(m), and every message is associated with a transaction.
Processes on the same node can communicate through \emph{shared base objects}.
The shared base objects are accessed through \emph{primitive operations}, which are predefined atomic operations on shared memory objects, such as read, write, read-modify-write (compare-and-swap, test-and-set, fetch-and-increment, etc.)
A primitive operation is said to be \emph{non-trivial} if it may modify the object. 

Formally, an implementation of a PDTS is a composition of I/O automatons as described in \cite{lynch96da}. We distinguish three types of I/O automatons: process, client, and channel I/O automatons. Besides the external actions of the form \emph{send(m)} and \emph{recv(m)}, which allow processes and clients to communicated with each other through the I/O channels (which model the network), processes can also be able to communicate through \emph{shared base objects} (which model the shared memory). We model the primitive operations used to access these shared base objects by introducing two new types of external actions: \emph{inout} actions, and \emph{outin} actions, which start as input, respectively output, actions, then instantly become output, respectively input, actions. Each shared base object is modeled as a I/O automaton with inout actions for every primitive operation it supports. Process I/O automatons access the shared objects through outin actions. The compositions rules remain the same, except that an outin transition is executed only if all shared object I/O automaton that has its action in their signature is able to execute the transition, i.e., the preconditions are all met. Thus, every primitive operation appears to have executed atomically. The first transition that each process is allowed to take is the one associated with a \emph{recv(m)} input action. All subsequent transitions are causally related to/triggered by a previous transition. The process does not take another \emph{recv(m)} transition until it reaches a \emph{final state} from which the only way to transition is through a \emph{recv(m)} action. We call the transition that brought the automaton to a final state, the \emph{final transition}, and intuitively it marks the end of the message handler.

Client I/O automatons additionally have internal actions of the form \emph{begin(T)}, \emph{read(T, K)},
\emph{write(T, K)}, \emph{commit(T)}, and \emph{abort(T)}, which simulate actions it receives from the application using the transactional interface. The first transition that each client is allowed to take is the one associated with \emph{begin(T)}, where T is a unique id of the current transaction being processed by this client. All subsequent actions (read, write, commit, abort) refer to the same T. The client does not take another \emph{begin(T)} transition until it reaches a \emph{final state} from which the only way to transition is through a \emph{begin(m)} action.

\smallskip\noindent
\textbf{Executions.} An \emph{execution} of an implementation of a PDTS is a sequence of 
%alternating states and
\emph{steps}.
%(similar to ~\cite{attiya2011inherent, peluso2015disjoint}). 
A step is associated with a transaction through a unique label, and can be of one of three types: 1) an \emph{intra-node communication} step is a primitive operation on a base object, 2) a \emph{transaction} step indicates the invocation (denoted \emph{b(egin)}), response (denoted \emph{r(esponse)}), or termination (either \emph{c(ommit)} or \emph{a(bort)}) of a transaction; a response step is the last step of the execution of a commit(t)/abort(t) operation; it returns the full read and write sets of the transaction and their order of execution (relative only to each other); a termination step, which discloses whether the transaction committed or aborted, is the last step of any transaction, and 3) an \emph{inter-node communication} step is a send(m)/receive(m) event or an end-of-handler event, e(oh), which is the last step of the message handler executed by the process. \footnote{ Note that, for more generality, the execution can be modeled as a \emph{partial order}, since certain steps can be taken in parallel and are impossible to order 
(for example, two processes on different nodes receiving messages at around the same time, or two processes executing in parallel primitive operations on different shared objects at around the same time), 
but, for our purposes, the arbitrary order picked between these steps is not important; all the other steps in the execution follow the real-time order. This practice is common in many previous works for simplicity reasons.}
Two primitive steps of an execution \emph{contend} on a base object $o$ if they both access $o$, and at least one of them applies a non-trivial primitive to $o$.

We use abstract \emph{version} numbers to relate the values returned by read operations to the write operations that generated them. Thus, each write operation is associated with a unique version number and each read operation is associated with a set of versions, $V$. $V$ may contain the initial version, $\perp$. If $V$ is empty then it means that the read operation returned a completely arbitrary value and if $V$ contains more elements then it means that the value returned by the read operation reflects the effects of multiple concurrent write operations.

We define the projection of $E$ on $T$, denoted as $E|T$, to be the subsequence of $E$ that consists of all the steps that are associated with $T$.  We define the projection of $E$ on a process $p$ and transaction $T$, denoted as $E|\{p,T\}$, to be the subsequence of $E$ that consists of all the steps associated with $T$ that were executed by process $p$.

\autoref{fig:execution_history} shows an example execution of three transactions, $T_1$, $T_2$, and $T_3$ (the last row in the figure). For simplicity, we stripped the complete execution of the states and many of the steps. 
For each transaction we maintained the invocation event, $b_{T_i}$, the primitive operations on shared base objects, $O_{T_i}(o_j)$, the events marking the response to the transaction invocation which are accompanied by the complete read and write sets of the transaction, and the events marking the termination of the transaction, $c_{T_i}$ or $a_{T_i}$ (the termination event happens after all the steps pertaining to the execution of the transaction; in this particular execution all transactions committed). The read and write sets contain operations of the form $R_{T_i}(X_j): V$ and $W_{T_i}(X_j, version)$, respectively, where $V$ is a set of versions as defined above. For every transaction $T_i$, the response event, $r_{T_i}$, happens in between its invocation event, $b_{T_i}$, and its termination event, $c_{T_i}$ and it may be the case that $r_{T_i}$ does not happen after all of $T_i$'s steps -- for example, there are implementations which try to reply to the client as soon as possible and asynchronously apply the transaction's updates (as is the case illustrated in the example execution in the figure).

\begin{figure*}[t!]
    \centering
    \includegraphics[scale=0.23]{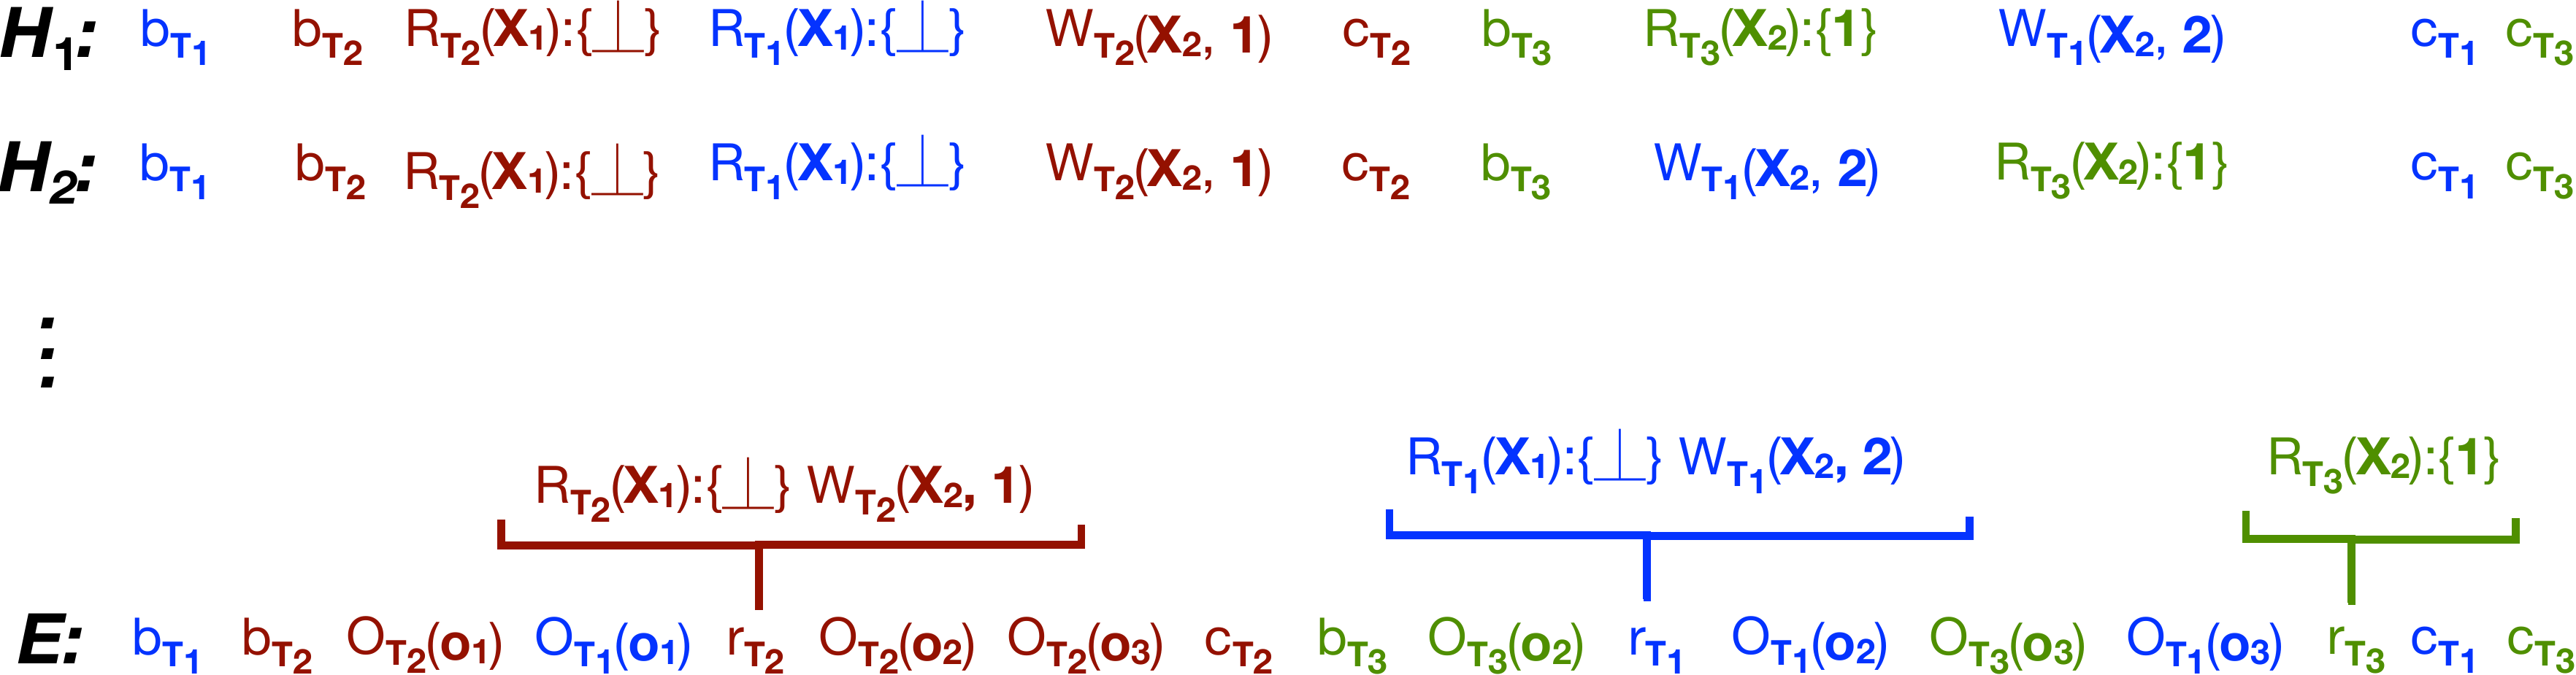}
    \caption{A simplified example of an execution, $E$, and two of its derived legal histories, $H_1$ and $H_2$. Steps pertaining to the execution of the same transaction are highlighted with the same color. The execution shows the processing of three transactions, $T_1$, $T_2$, and $T_3$. $T_1$ executed concurrently with the other two, while $T_2$ terminated before $T_3$. The derived histories preserve the order of transactions that did not execute concurrently (and their operations). For concurrent transactions, the histories propose an arbitrary order between their operations, while still preserving the order of operations within the same transaction as returned by the response events, $r_{T_i}$. }
    \label{fig:execution_history}
    \vspace{-1mm}
\end{figure*}

\smallskip\noindent
\textbf{Traces.} A \emph{trace} of an execution $E$ is the subsequence of $E$ consisting of all the inter-node communication steps.

\smallskip\noindent
\textbf{Histories.}
A \emph{history} (similar to the one defined in ~\cite{bernstein86cc}) is a higher-level model of an execution defined as a sequence of read and write operations of the transactions that executed, together with the respective begin and termination events. Starting from an execution, a history is \emph{derived} by stripping the execution of all states, primitive operations, and send and receive message events, and replacing the response events with the the read and write operations they returned. The order of the begin and termination events is preserved in the history, as well as the orders returned by the response events. Two transactions executed \emph{concurrently} if the time interval between their invocation and termination events overlaps. In \autoref{fig:execution_history} transaction $T_1$ executed concurrently with both $T_2$ and $T_3$, while $T_2$ executed before $T_3$. The order of the read and write operations of transactions that did not execute concurrently is also preserved in the history. For concurrent transactions, an arbitrary order is picked between their operations, which indicates that multiple possible histories can be derived from the execution. In \autoref{fig:execution_history} we illustrate two possible derived histories, $H_1$ and $H_2$, from the same execution, $E$ (more are possible).

We say that a history is \emph{legal} if each read operation of each committed transaction reflects the effects of an atomic write operation. Formally, each read operation of each committed transaction is associated with a version set that contains exactly one element, which is either $\perp$, or the version used by a previous write operation.
In \autoref{fig:execution_history} both derived histories are legal. A \emph{serial} history is a legal history where for every two transactions that appear in the history, either all operations of the first one appear before all operations of the second one or vice versa. %\Naama{I'm wondering whether matching the sequential specification is what is needed to map an execution to a history. In that case, we should talk about this earlier in this paragraph.}
Two histories are \emph{equivalent} if they contain the same transactions and their same operations and they order conflicting operations of committed transactions in the same way. The \emph{serialization graph} for a legal history, \emph{H}, is a directed graph whose nodes are the transactions that are committed in the history and whose edges are all $T_i \rightarrow T_j$ ($i \neq j$) such that one of $T_i$'s operations precedes and conflicts with one of $T_j$'s operations in \emph{H}.

%\Naama{I think this entire previous sentence should refer to \emph{legal} histories only.} \aaasz{fixed}

\textbf{Serializability.} The preferred correctness property for most of the transactional systems is \emph{serializability}, which prescribes that transactions appear to have executed serially, one after the other. Formally, an implementation of a PDTS satisfies \emph{serializability} if from every execution it produces it can be derived a history that is equivalent to a serial history.

\textbf{Weak progress.} A transactional system should at least guarantee weak progress: in all failure-free executions every transaction that did not execute concurrently with any other transaction, terminates successfully (commits).

%We are interested in the time it takes for processes to terminate in `good' executions. We consider an execution to be \emph{good} if it is \emph{synchronous} and \emph{failure-free}. \Naama{Need to think more carefully here. Failure-freedom is assumed for the non-replicated case anyway, I think.} We call such executions \emph{well-behaved}. Given an algorithm that tolerates asynchrony, we ask how many rounds are needed in a well-behaved execution until the client knows the result of its transaction, starting from the first non-trivial message sent by $c$.
%\Naama{We can rely on Lamport's notion of message delays from fast paxos, or communication steps from Keidar and Rajsbaum}

\textbf{Failure model.} Nodes can fail by crashing; if a node crashes then \emph{all} processes on the node crashed as well. We do not consider failures where individual processes crashed and we assume clients do not fail. We denote \emph{failure-free} execution to be an execution where no node crashed.

%\aaasz{TODO: do we need to define fault-tolerance here?}
%\Naama{Define fault tolerance, mention that clients and processes don't fail, only nodes.}
